# Supplementary material for: Neural Collapse in Multi-label Learning with Pick-all-label Loss
Source: arXiv:2310.15903 source file (2024-06-20)
Supplement: Supplementary file 1 [file app_exp.tex]

% The detailed information of SVHN dataset are included in \Cref{fig:svhn_setup}
% \begin{figure}[t]
%     \centering
%     \subfloat[The SVHN Dataset]{\includegraphics[width=0.44\textwidth]{figures/SVHN_demo.png}} \
%     \hspace{0.1in}
%     \subfloat[Class Distribution]{\includegraphics[width=0.44\textwidth]{figures/svhn_mul_2_dist.png}} \
%     \caption{\textbf{Our usage of the SVHN dataset.} As illustrated in (a), the Street View House Numbers (SVHN) Dataset \citep{netzer2011reading} comprises labeled numerical characters and inherently serves as a multi-label learning dataset. We applied minimal preprocessing to achieve balance specifically within the Multiplicity-1 scenario, as evidenced by the diagonal entries in (b). Furthermore, we omitted samples with Multiplicity-4 and above, as these images posed considerable recognition challenges. Notably, the Multiplicity-2 case remained largely imbalanced, as observed in the off-diagonal entries in (b). Nonetheless, our findings remained robust and consistent in this scenario, as evidenced in \Cref{fig:NC-SVHN}.
%     }
%     \label{fig:svhn_setup}
% \end{figure}
